# Supplementary material for: Composite Optimization with Error Feedback: the Dual Averaging Approach
Source: arXiv:2510.03507 source file (2025-10-03)
Supplement: Supplementary file 1 [file prox-real-iterates.tex]

\section{Analysis of the Proximal \algname{EControl}}
\label{sec:analysis-proximal-econtrol}
